# Supplementary material for: Matryoshka: Stealing Functionality of Private ML Data by Hiding Models in Model
Source: arXiv:2206.14371 source file (2022-06-29)
Supplement: Supplementary file 1 [file appendix.tex]

\appendix
\section{Omitted Technical Proofs}
\label{sec:appendix:proof}

\section{Omitted Algorithmic Details}
\label{sec:appendix:algorithm}
We provide the detailed algorithms for \textbf{Fill}, \textbf{Propagate}, \textbf{Decode} in Algorithm \ref{alg:fill} \& \ref{alg:decode} respectively.

\section{More Evaluation Details \& Results}
\label{sec:appendix:exp}
\subsection{Details on the Metrics on Data Stealing}
We use the following metrics to measure the effectiveness of data stealing. 
\begin{itemize}
    \item \textbf{Mean Square Error} (\textit{MSE}): MSE measures the $L_{2}$ difference between the reconstructed sample and the ground-truth sample after being averaged over coordinates. In image domain, MSE represents pixel-wise error. In audio domain, MSE represents frame-wise error. Formally, MSE writes $\operatorname{MSE}(\hat{x},x) =||\hat{x}-x||_{2}/\operatorname{dim}(x)$, where $\operatorname{dim}(x)$ is the dimension of the sample. A lower MSE implies more effective data stealing.
    \item \textbf{Structural Similarity Index} (\textit{SSIM}): SSIM\cite{wang2004image} measures the structural similarity between the reconstructed image and the ground-truth image, while incorporating perceptual phenomena, including luminance and contrast, as well. It formally computes as
   $
        \text{SSIM}(x, \hat{x})=\frac{\left(2 \mu_{x} \mu_{\hat{x}}+c_{1}\right)\left(2 \sigma_{x \hat{x}}+c_{2}\right)}{\left(\mu_{x}^{2}+\mu_{\hat{x}}^{2}+c_{1}\right)\left(\sigma_{x}^{2}+\sigma_{\hat{x}}^{2}+c_{2}\right)},
$
where the mean of x$(\mu_{x})$ stands for luminance, the variance of x$(\sigma_{x})$ stands for contrast and covariance$(\sigma_{x \hat{x}})$ stands for structural information. SSIM ranges from 0 to 1. A higher SSIM implies more effective data stealing.
\end{itemize}

%%%%% on stealing the non-learnable parameters

\subsection{Details on the Secret Tasks}
\begin{table}[H]
\centering
\caption{Datasets and architectures.}
\label{tab:datasets}
\scalebox{0.8}{
\begin{tabular}{lll}
\toprule
Dataset & Task & Architecture \\
\midrule
CIFAR-10 \cite{krizhevsky2009learning}& Object Classification & ResNet-18 \cite{he2016deep} \\
GTSRB \cite{Houben-IJCNN-2013} & Traffic Sign Recognition & VGG-16 \cite{simonyan2014very}\\
DermaMNIST \cite{medmnistv2}& Skin Cancer Diagnosis & LeNet-5\cite{lecun1998gradient}\\
IMDB \cite{maas-EtAl:2011:ACL-HLT2011}& Sentiment Classification & TextCNN \cite{zhang2015sensitivity}\\
SpeechCommand \cite{speechcommandsv2} &Speech Recognition&M5 \cite{7952190}\\
Warfarin \cite{Truda2020warfit}& Dose Estimation&MLP \\
VOC'07 \cite{Everingham15}& Object Detection &MoblieNetV2-SSD\cite{howard2017mobilenets} \\
UWave \cite{liu2009uwave}& Time Series Classification &RNN \\
\bottomrule
\end{tabular}}
\end{table}
Table \ref{tab:datasets} summarizes the basic information of the datasets, tasks and architectures used in our evaluation. We provide more details below.

\noindent\textbf{Image Domain.}
\begin{itemize}
    \item \textbf{CIFAR-10 \cite{krizhevsky2009learning}:} CIFAR-10 consists of 60,000 32$\times$32 RGB images, which covers 10 daily objects of different categories. It is widely used as a benchmark for image classification. The standard model we used is ResNet-18\cite{he2016deep}, which has 11.17M parameters in total.
    \item \textbf{GTSRB \cite{Houben-IJCNN-2013}:} German Traffic Sign Benchmark Dataset (GTSRB) is composed of over 50,000 32$\times$32 RGB images of 43 different traffic signs, which simulates an image recognition scenario in self-driving cars. The model we use is VGG-16\cite{simonyan2014very}, which is made of 14.74M parameters in total. 
    \item \textbf{VOC'07 \cite{Everingham15}:} Visual Object Classes 2007 (VOC'07) dataset has 300$\times$300 RGB images of 20 classes, which is commonly used for the object detection task. It consists of 9,963 images in total, containing 24,640 annotated objects. We fit it with a model called MobileNetV1-SSD \cite{howard2017mobilenets} of 9.47M parameters.
\end{itemize}
\noindent\textbf{Text Domain.}
\begin{itemize}
    \item \textbf{IMDB \cite{maas-EtAl:2011:ACL-HLT2011}:} IMDB dataset has 50,000 movie reviews, which is commonly used in natural language processing tasks. In our evaluation, it is used for sentiment classification task. We use TextCNN\cite{zhang2015sensitivity} as the secret model, which has 6.69M parameters in total.
\end{itemize}
\noindent\textbf{Audio Domain.}
\begin{itemize}
    \item \textbf{SpeechCommand \cite{speechcommandsv2}:} SpeechCommand is a dataset of 35 different voice commands spoken by different people, which has over 100,000 1 second long audio files with a sampling frequency of 16kHz. We use M5\cite{7952190} of 26.92K parameters to conduct the speech command classification task.
    % 105829 11005
\end{itemize}
\noindent\textbf{Time Series Domain.}
\begin{itemize}
    \item \textbf{UWave \cite{liu2009uwave}:} UWave dataset is a large gesture library with over 4,000 samples collected from eight users over an elongated period of time, which is used to recognize 8 different gesture patterns identified by a Nokia research. We use an RNN of 1.67K parameters as the standard model.
\end{itemize}
\noindent\textbf{Healthcare Domain.}
\begin{itemize}
    \item \textbf{Warfarin \cite{Truda2020warfit}:} Warfarin is a dataset that contains 6,256 patients' medical records, which is used for the warfarin dose estimation task. The records not only contain patients' basic information like gender, race, age, weight, height etc., but also contain pathology information like VKORC1 Genotype, CYP2C9 Genotype Count etc. We fit it with an MLP containing 0.5K parameters.
    \item \textbf{DermaMNIST \cite{medmnistv2}:} DermaMNIST consists of over 10,000 images of pigmented skin lesions taken  by dermatoscope, which are categorized into 7 classes. It is commonly treated as an image classification task. For convenience, we resize the images to 32$\times$32 RGB format and fit the task with LeNet-5 \cite{lecun1998gradient} of 61.98K parameters.
\end{itemize}

We measure the performance on each dataset and task with the standard evaluation protocol accordingly. We provide more details below.
\begin{itemize}
    \item \textbf{ACC}: Accuracy (ACC) is the standard evaluation metric for classification tasks. ACC measures the proportion of correctly predicted samples. It formally writes $\operatorname{ACC} = \frac{\sum_{i=1}^{N} \mathbf{1}\{f(x_{i})=y_{i}\}}{N} $, where $N$ is the total number of the test samples.
    \item \textbf{MAP}: Mean average precision (MAP) is the common evaluation metric for the object detection task, which is the average of AP (average precision) over all object classes.
    \item \textbf{MSE}: Mean Square Error (MSE) measures the $L_{2}$ difference between the predicted output and the ground-truth output after being averaged over the coordinates. Formally, MSE writes $\operatorname{MSE}(f(x),y) =||f(x)-y||_{2}/\operatorname{dim}(y)$, where $\operatorname{dim}(y)$ is the dimension of the ground-truth output. 
\end{itemize}

%%%%%%%%%%%%% BEGIN OF Defense Suite
\begin{figure}[t]
\begin{center}
\includegraphics[width=0.45\textwidth]{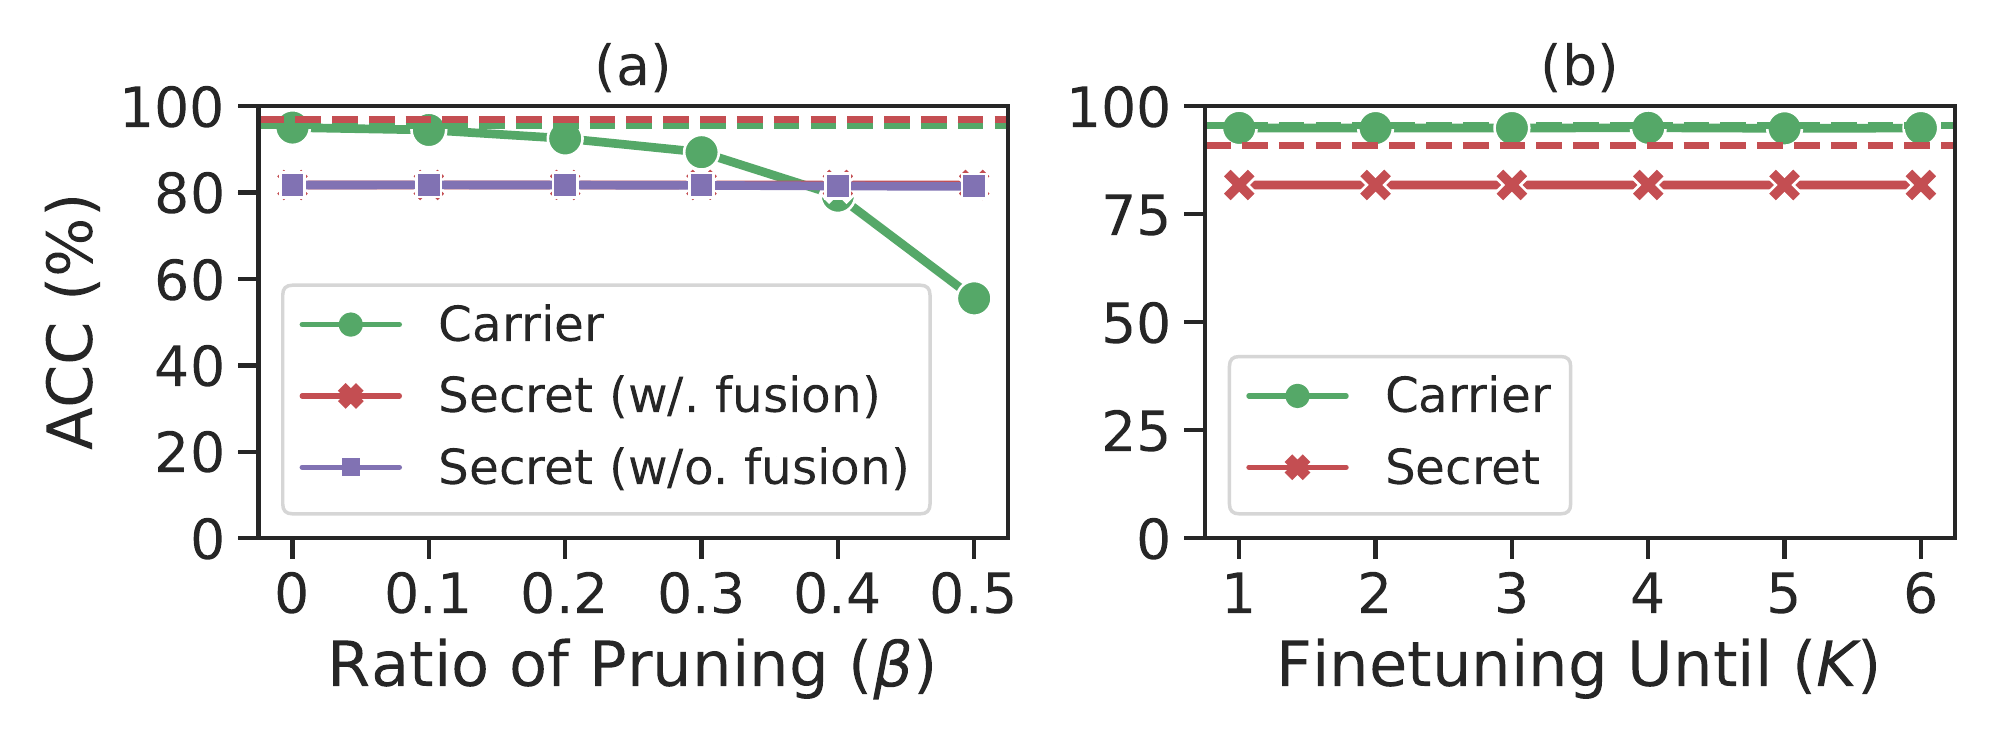}
\caption{Performance of the carrier/secret models under different levels of (a) weight pruning and (b) model finetuning on IMDB.}
\label{fig:defense_textcnn}
\end{center}
\end{figure}
%%%%%%%%%%%%%% END OF Defense Suite

%%%%%%%%%%%%% BEGIN OF Defense Suite
\begin{figure}[t]
\begin{center}
\includegraphics[width=0.45\textwidth]{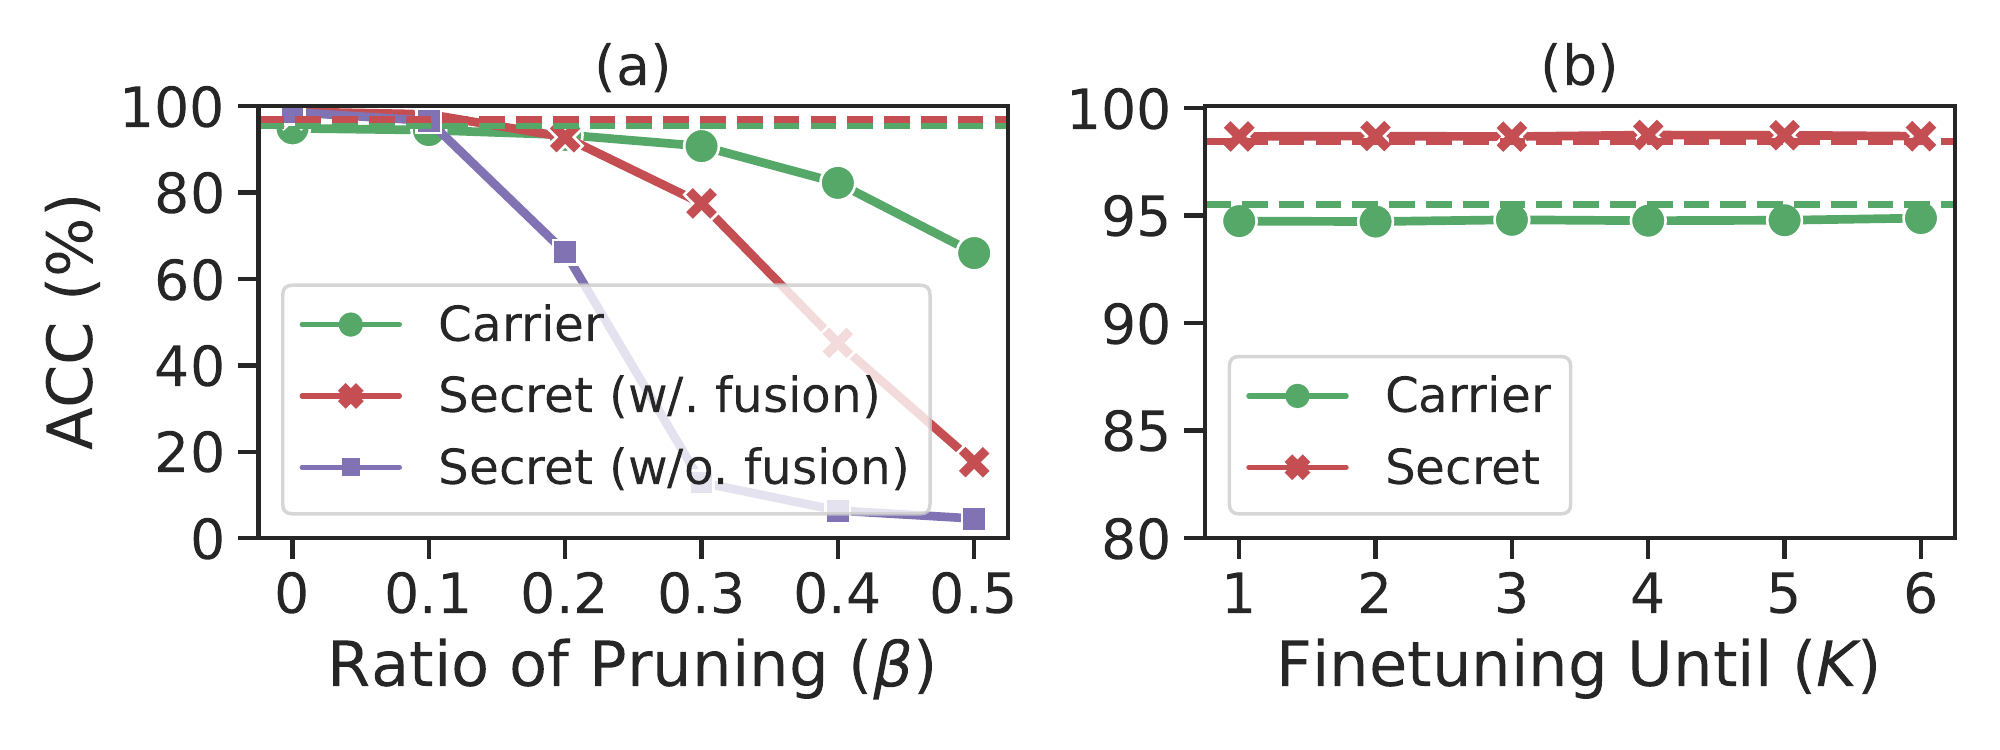}
\caption{Performance of the carrier/secret models under different levels of (a) weight pruning and (b) model finetuning on GTSRB.}
\label{fig:defense_vgg}
\end{center}
\end{figure}
%%%%%%%%%%%%%% END OF Defense Suite

\subsection{More Evaluation Results}
We also evaluate the effectiveness of data stealing on CIFAR-10 and SpeechCommand. As Fig.\ref{fig:cifar_ssim_bar} shows, Matryoshaka can steal over 10000 CIFAR-10 images with an SSIM uniformly higher than $0.85$ with only $0.5\%$ accuracy drop on the carrier model, which substantially outperforms the existing attack. Furthermore, due to model capacity limitations, Sign and Covariance encoding cannot be conducted when N reaches 512, 4096 respectively. And when $N=12288$, LSB encoding will cause the accuracy of the carrier model to drop drastically. The qualitative comparison between our attack and the Covariance and Sign Encoding when stealing 128 random data samples from CIFAR-10 is shown in Fig.\ref{fig:cifar_visual}, where our reconstructed images are perceptually indistinguishable with the ground-truth ones and far better than the reconstructed ones in the existing attack.

\begin{figure}[ht]
\begin{center}
\includegraphics[width=0.4\textwidth]{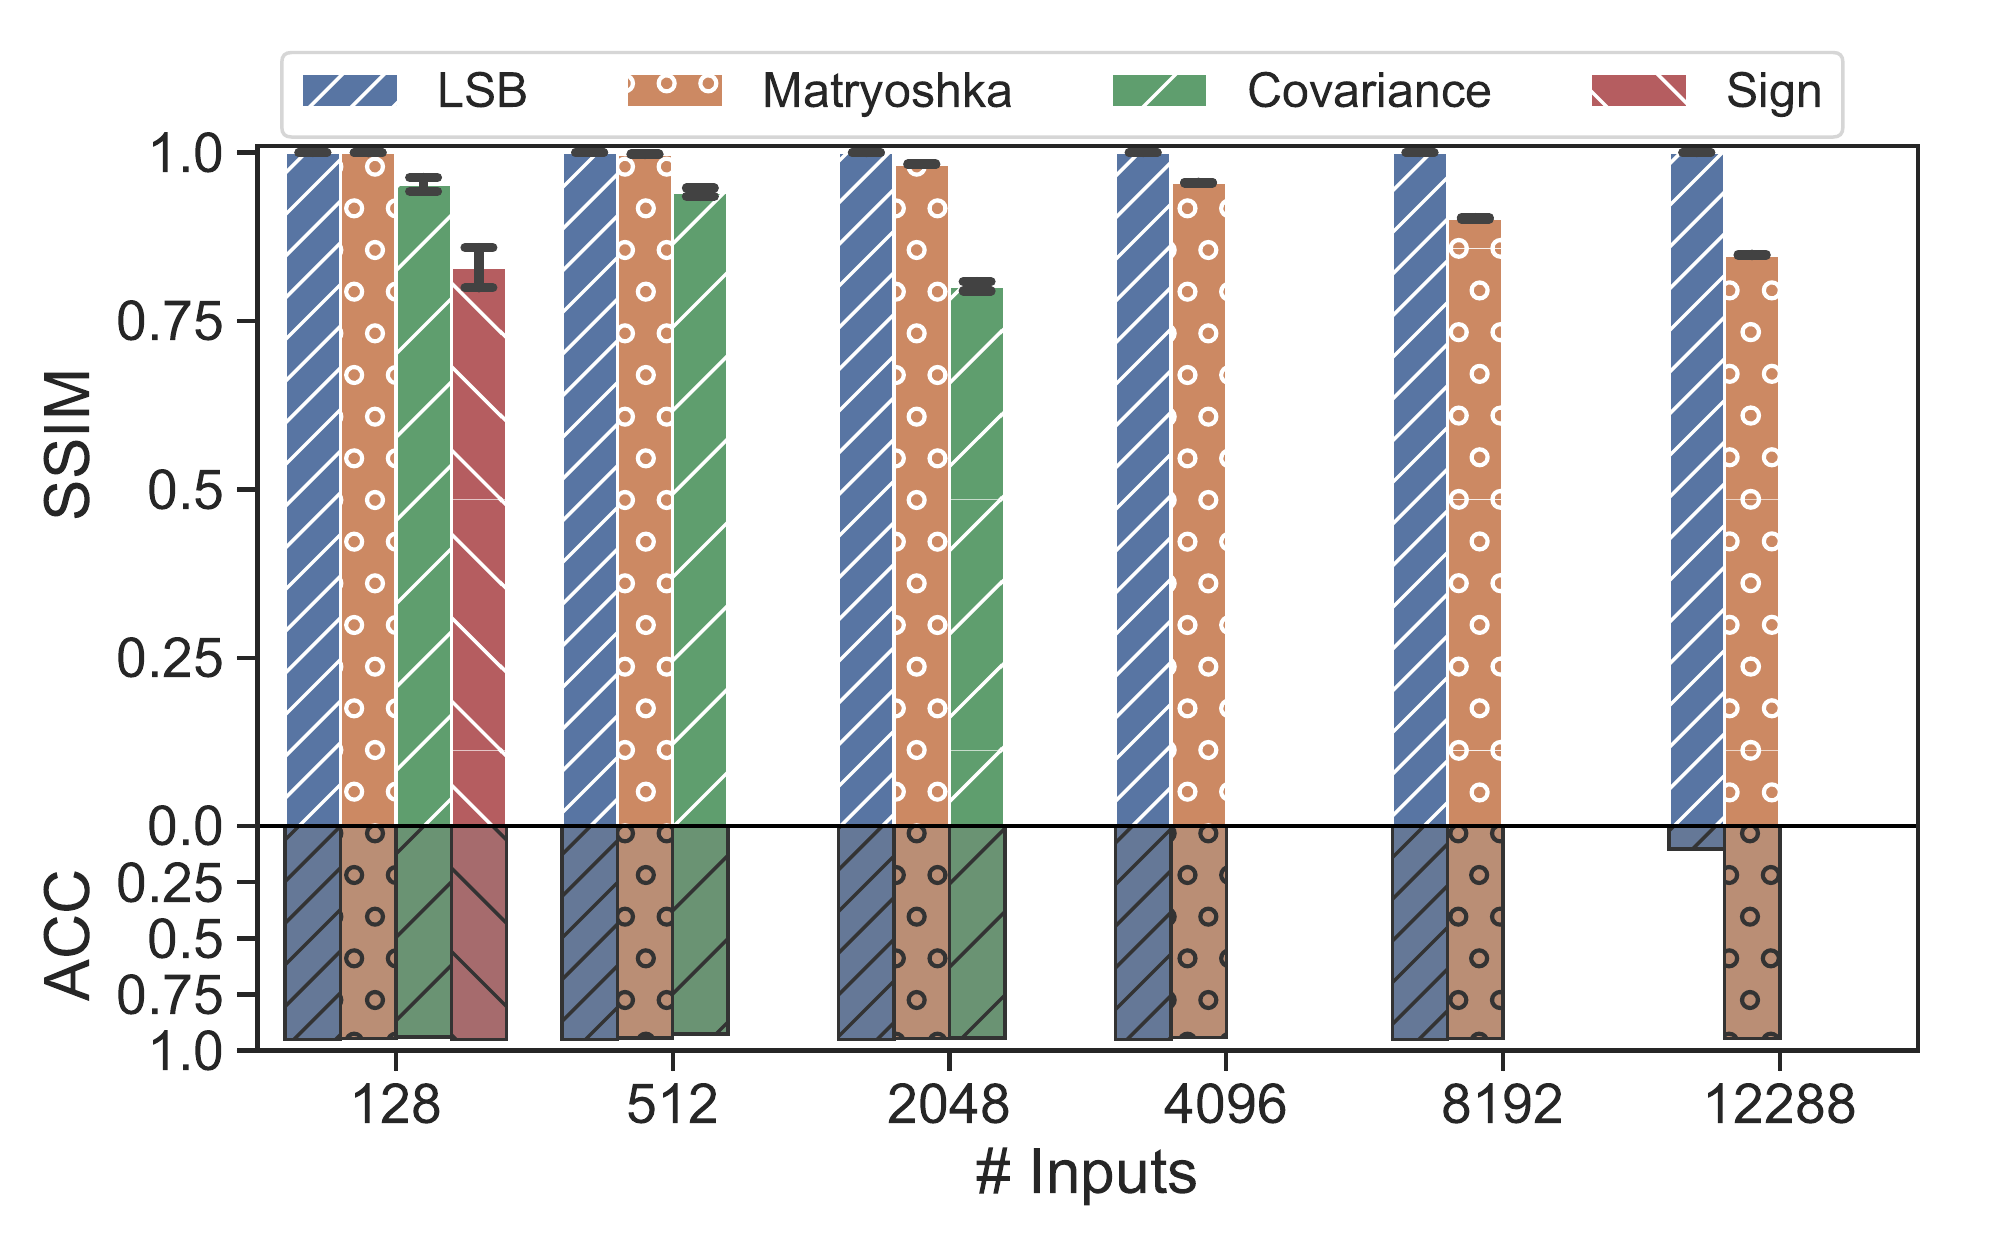}
\caption{The effectiveness of data stealing in terms of SSIM and the accuracy of the carrier model when the number of targets inputs continually increase on CIFAR-10.}
\label{fig:cifar_ssim_bar}
\end{center}
\end{figure}

\begin{figure}[ht]
\begin{center}
\includegraphics[width=0.45\textwidth]{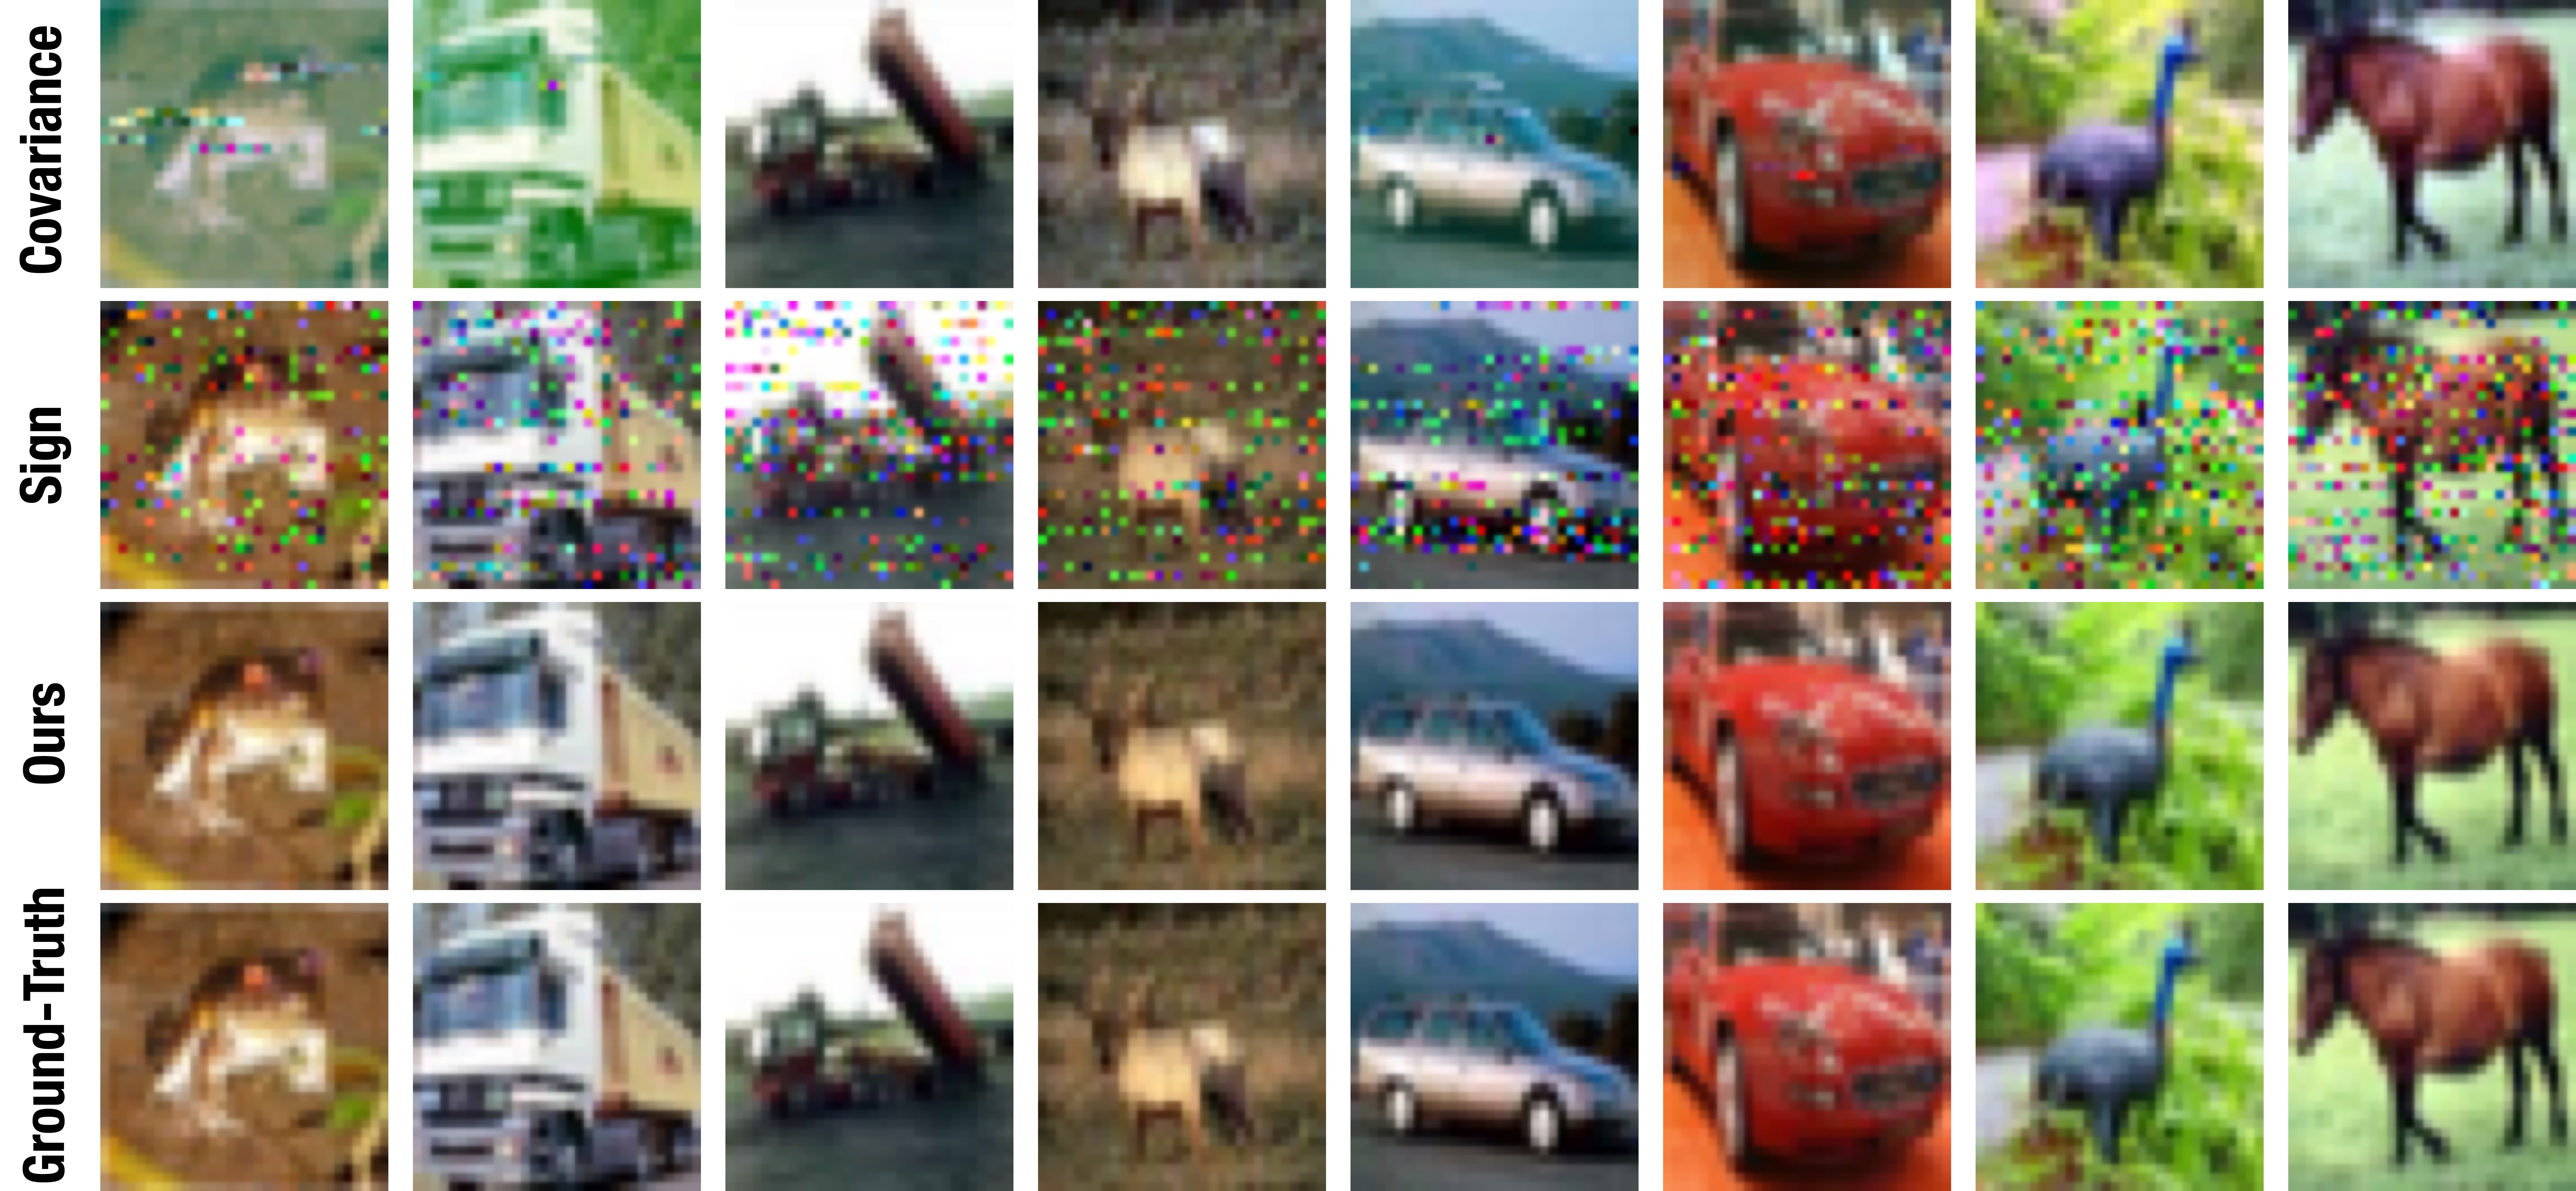}
\caption{Sampled results on CIFAR-10 with different data stealing approach.}
\label{fig:cifar_visual}
\end{center}
\end{figure}

As Table. \ref{tab:speech} shows, Matryoshaka can steal over 4000 audios with the MSE loss uniformly lower than $5\times{10}^{-4}$ on each frame with less than $0.5\%$ accuracy drop on the carrier model. This proves that our data stealing attack is flexible enough to be conducted not only on the image domain, but also on other domains. The waveform comparison between reconstructed audios and ground-truth audios when stealing 256 random audio samples is shown in Fig.\ref{fig:voice_visual}.
% Table generated by Excel2LaTeX from sheet 'Sheet1'
\begin{table}[htbp]
  \centering
  \label{speechcommand}
  \caption{The effectiveness of data stealing in terms of SpeechCommand}
    \begin{tabular}{ccc}
    \toprule
    \multirow{2}[4]{*}{\textbf{\# Inputs}} & \multicolumn{2}{c}{\textbf{Matryoshka}} \\
\cmidrule{2-3}          & MSE   & Acc \\
    \midrule
    256   & 0.000150028 & 95.15\% \\
    512   & 0.000269945 & 95.07\% \\
    1024  & 0.000350233 & 95.31\% \\
    2048  & 0.000424155 & 95.09\% \\
    4096  & 0.000488342 & 95.15\% \\
    \bottomrule
    \end{tabular}%
  \label{tab:speech}%
\end{table}%

\begin{figure}[ht]
\begin{center}
\includegraphics[width=0.45\textwidth]{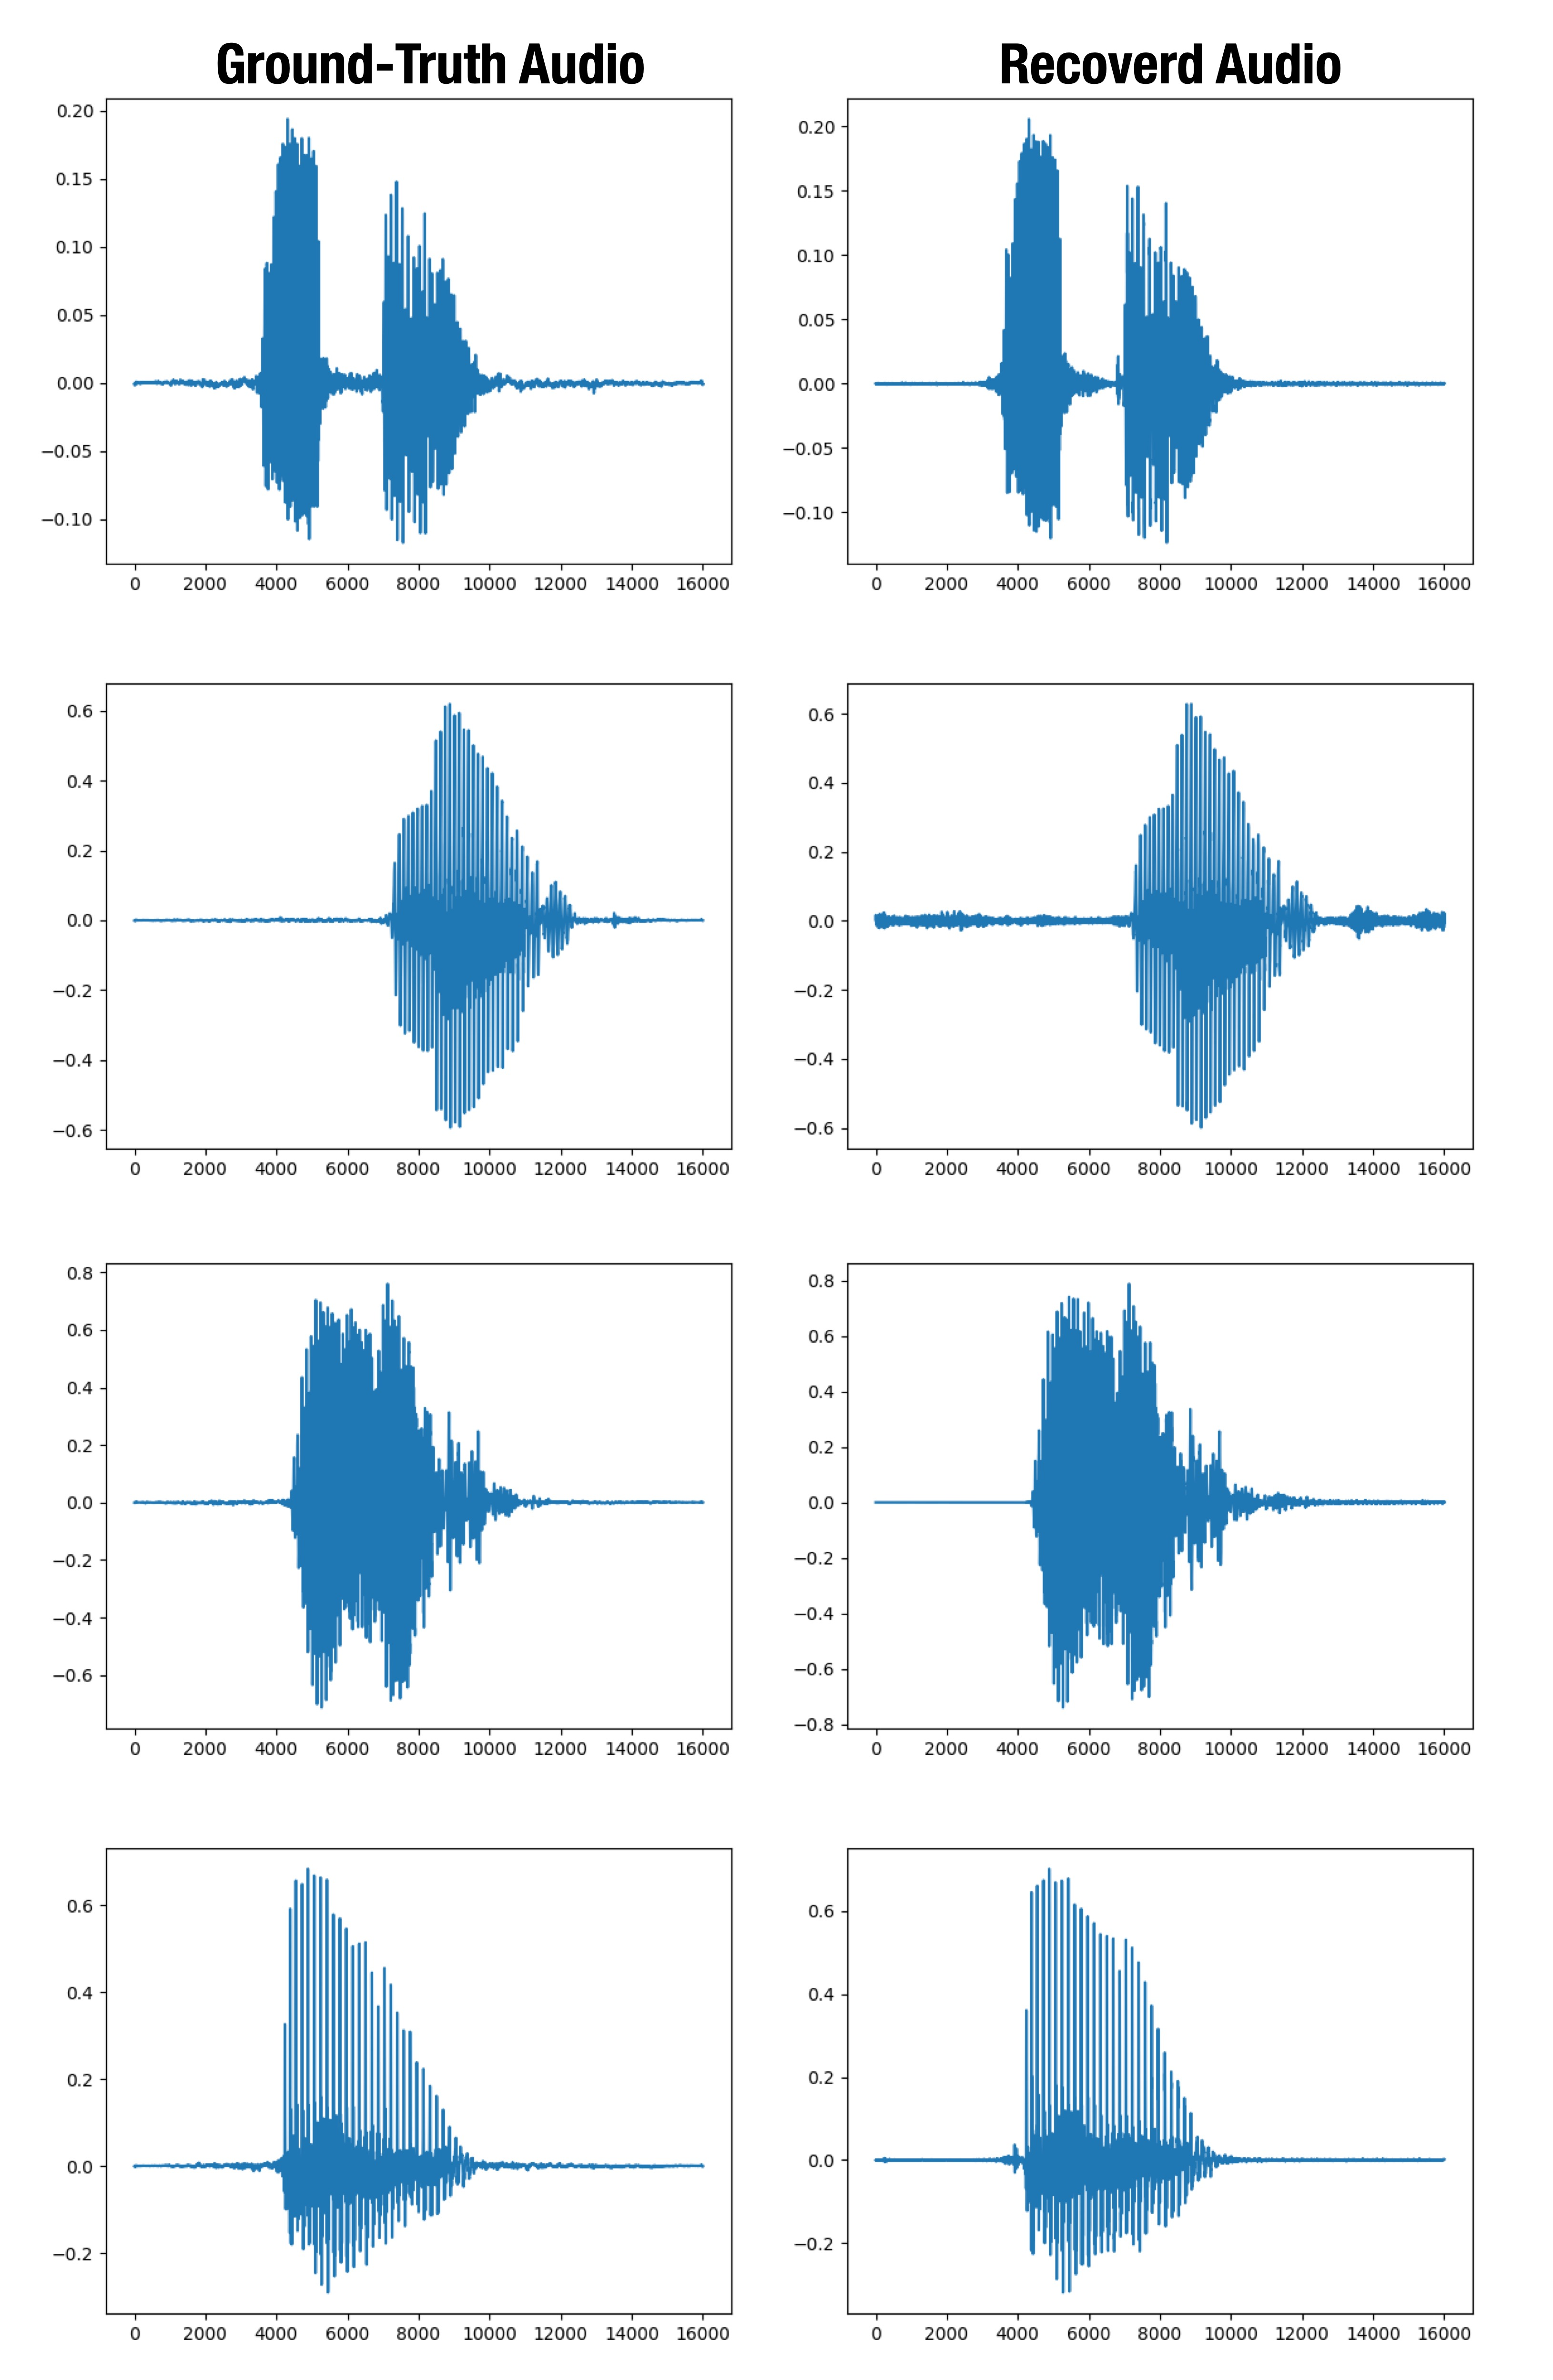}
\caption{Sampled waveform results on SpeechCommand when stealing 256 random audios.}
\label{fig:voice_visual}
\end{center}
\end{figure}
